# Supplementary material for: Limits on Optical Counterparts to the Repeating FRB 20180916B from High-speed Imaging with Gemini-N/'Alopeke
Source: arXiv:2311.09316 source file (2023-11-15)
Supplement: Supplementary file 1 [file appendix.tex]

\appendix

\section{XX}
\label{sec:xx}
XXX
\subsection{XX}

XXX
